# Supplementary material for: Semantic Layout Manipulation with High-Resolution Sparse Attention
Source: arXiv:2012.07288 source file (2022-04-15)
Supplement: Supplementary file 1 [file appendix_cvpr.tex]

\twocolumn[{%
 \centering
 \large \textbf{Supplementary Material for Semantic Layout Manipulation with High-Resolution Sparse Attention} \\[1.5em]
}]

% \onecolumn
% \section{Appendix}
%In this supplementary material, we provide 
%more qualitative comparisons in Sec.~\ref{sec:visual},
%visualization of the learned correspondence in Sec.~\ref{sec:correspondence},
%the reference-based layout manipulation in Sec.~\ref{sec:ref-based}, comparison against %more approaches in Sec.~\ref{sec:compare},
%and more implementation details in Sec.~\ref{sec:paper}.

\setcounter{section}{0}
\section{More Qualitative Comparisons}
\label{sec:visual}
In Fig.~\ref{fig:compare_manipulation} and Fig.~\ref{fig:compare_guided_inpainting}, we provide more qualitative comparisons on the image manipulation and the guided reconstruction task on the Place365 dataset, respectively. In Fig.~\ref{fig:compare_real_manipulation}, we show more image manipulation results on real data and visualize the intermediate warping results of our model in comparison to CoCosNet~\cite{supp_cocosnet}.

\begin{figure*}[h]
	\centering
	\includegraphics[width=0.85\linewidth]{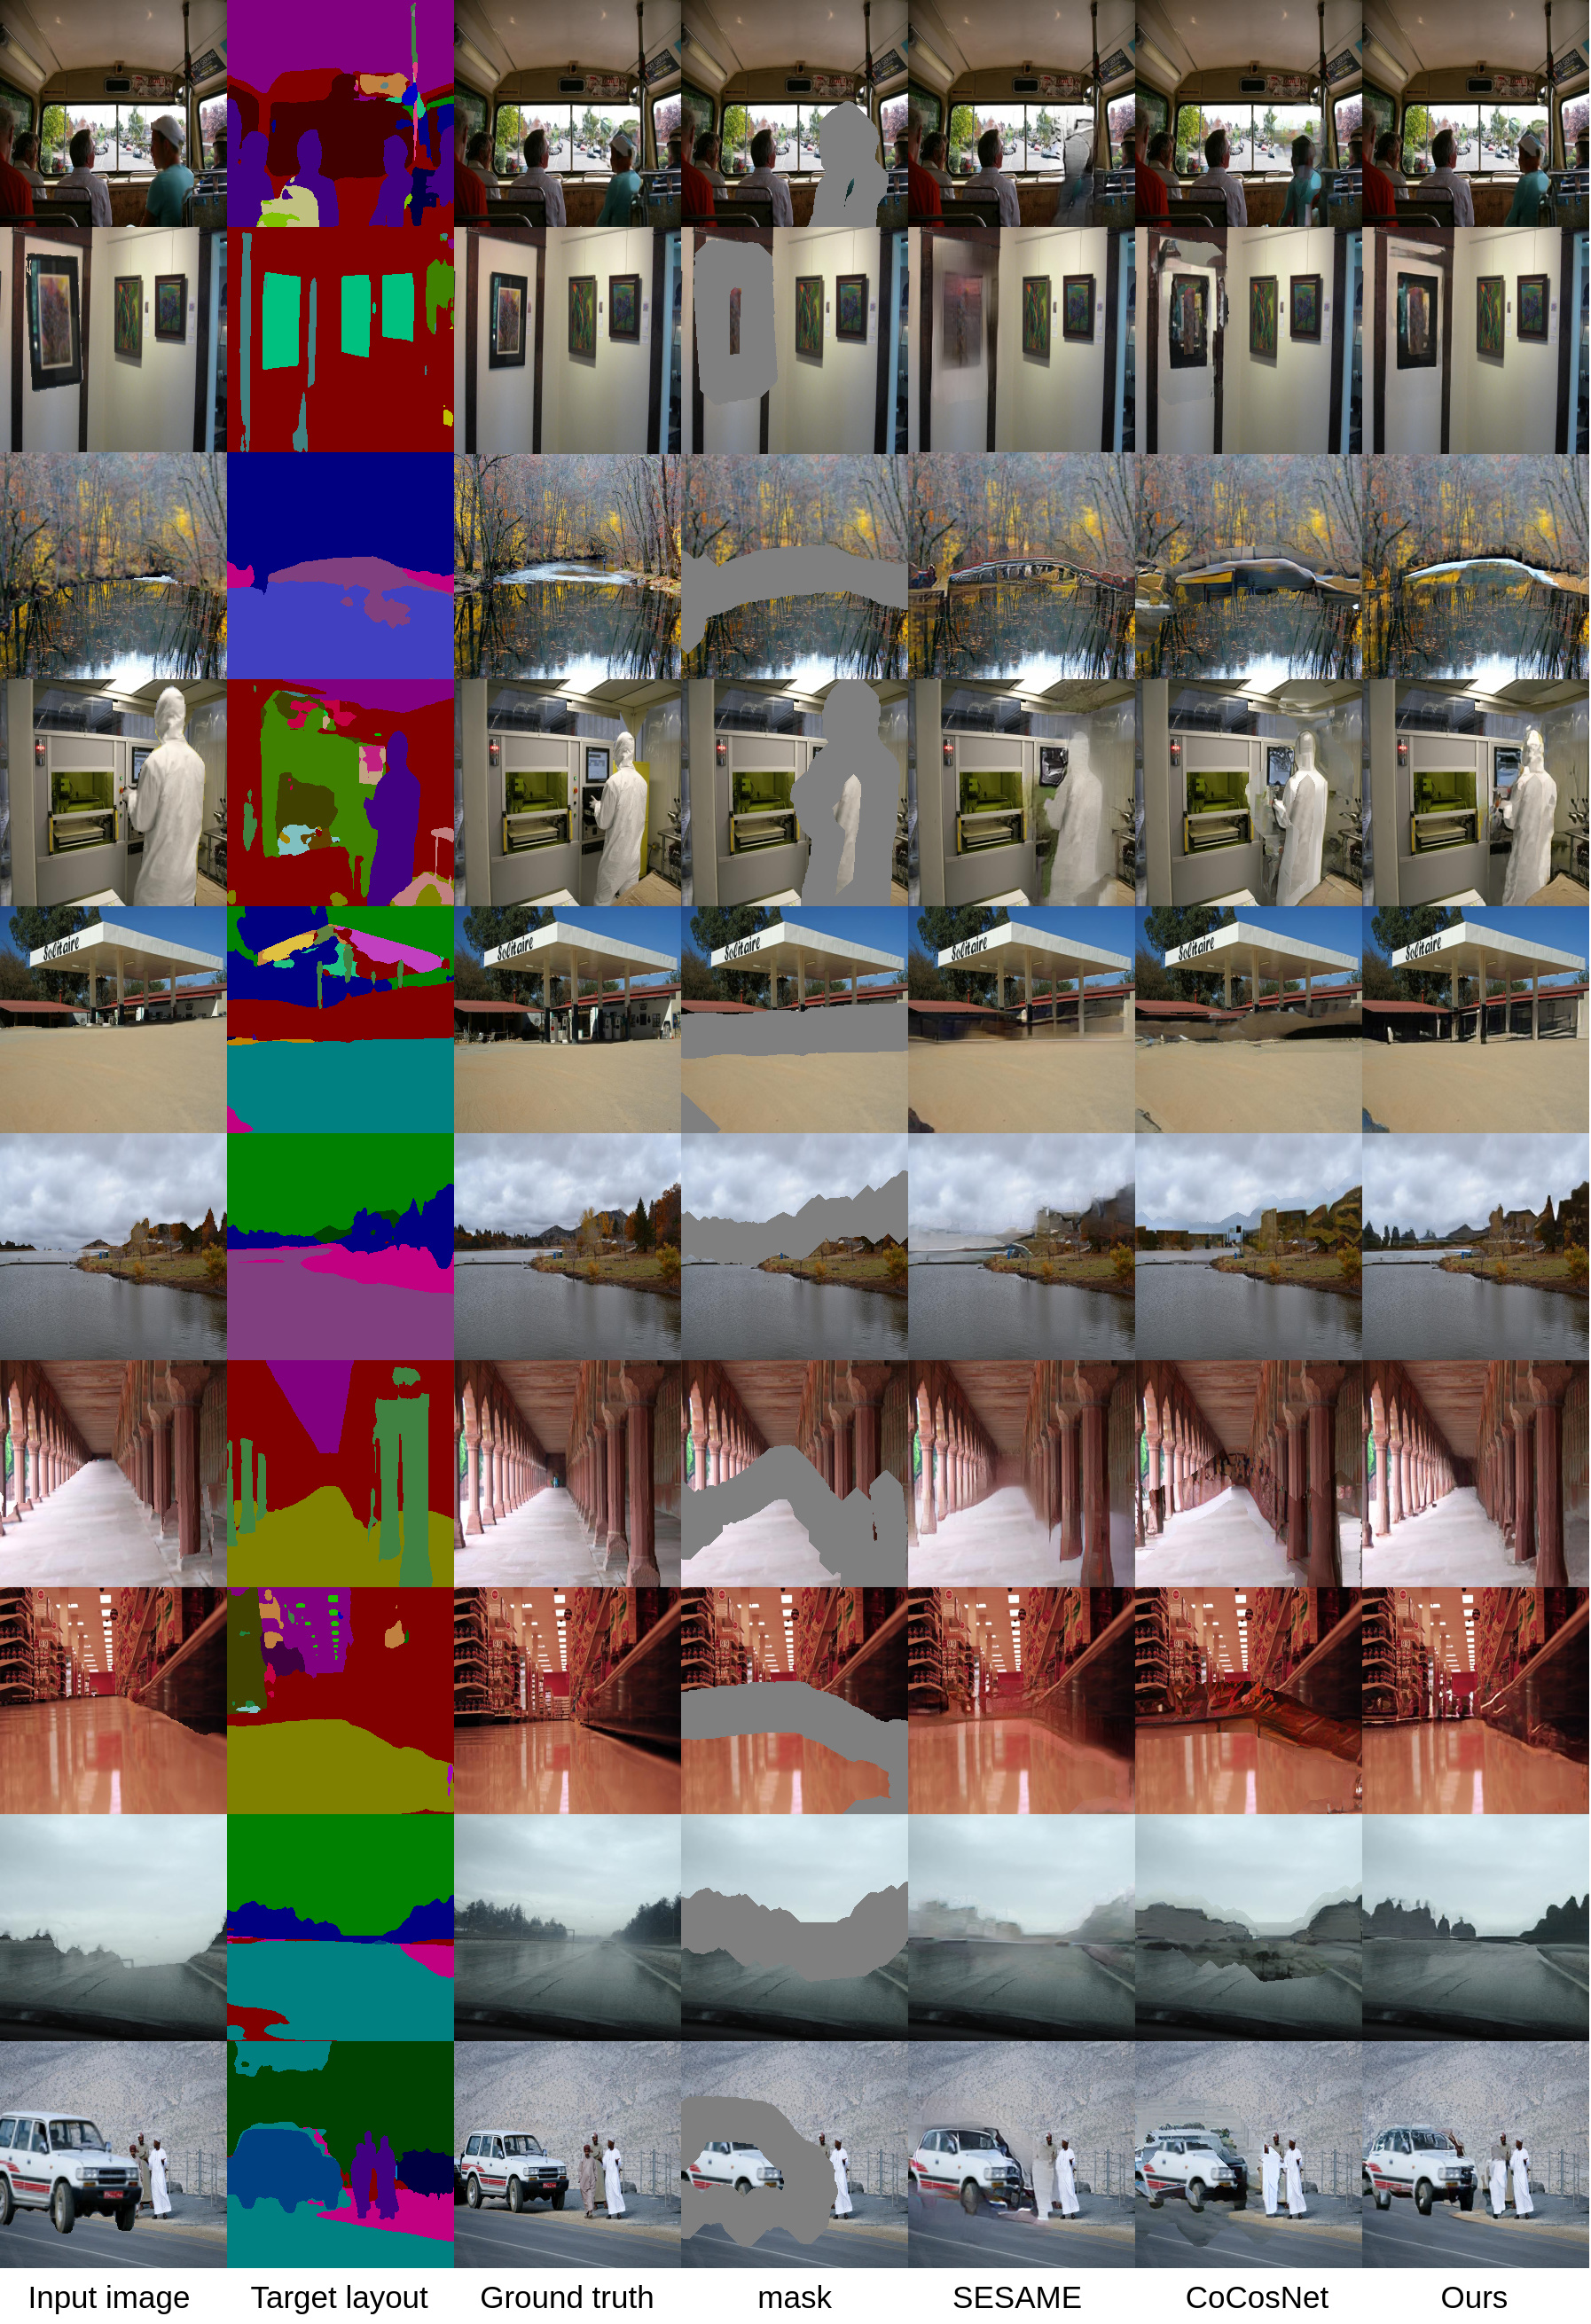}
	\caption{
	\textbf{Qualitative comparisons on the image manipulation task (Places365 dataset).} Best viewed (e.g. local textures) with zoom-in on screen.}
	\label{fig:compare_manipulation}
\end{figure*}

\begin{figure*}[t]
	\centering
	\includegraphics[width=1.0\linewidth]{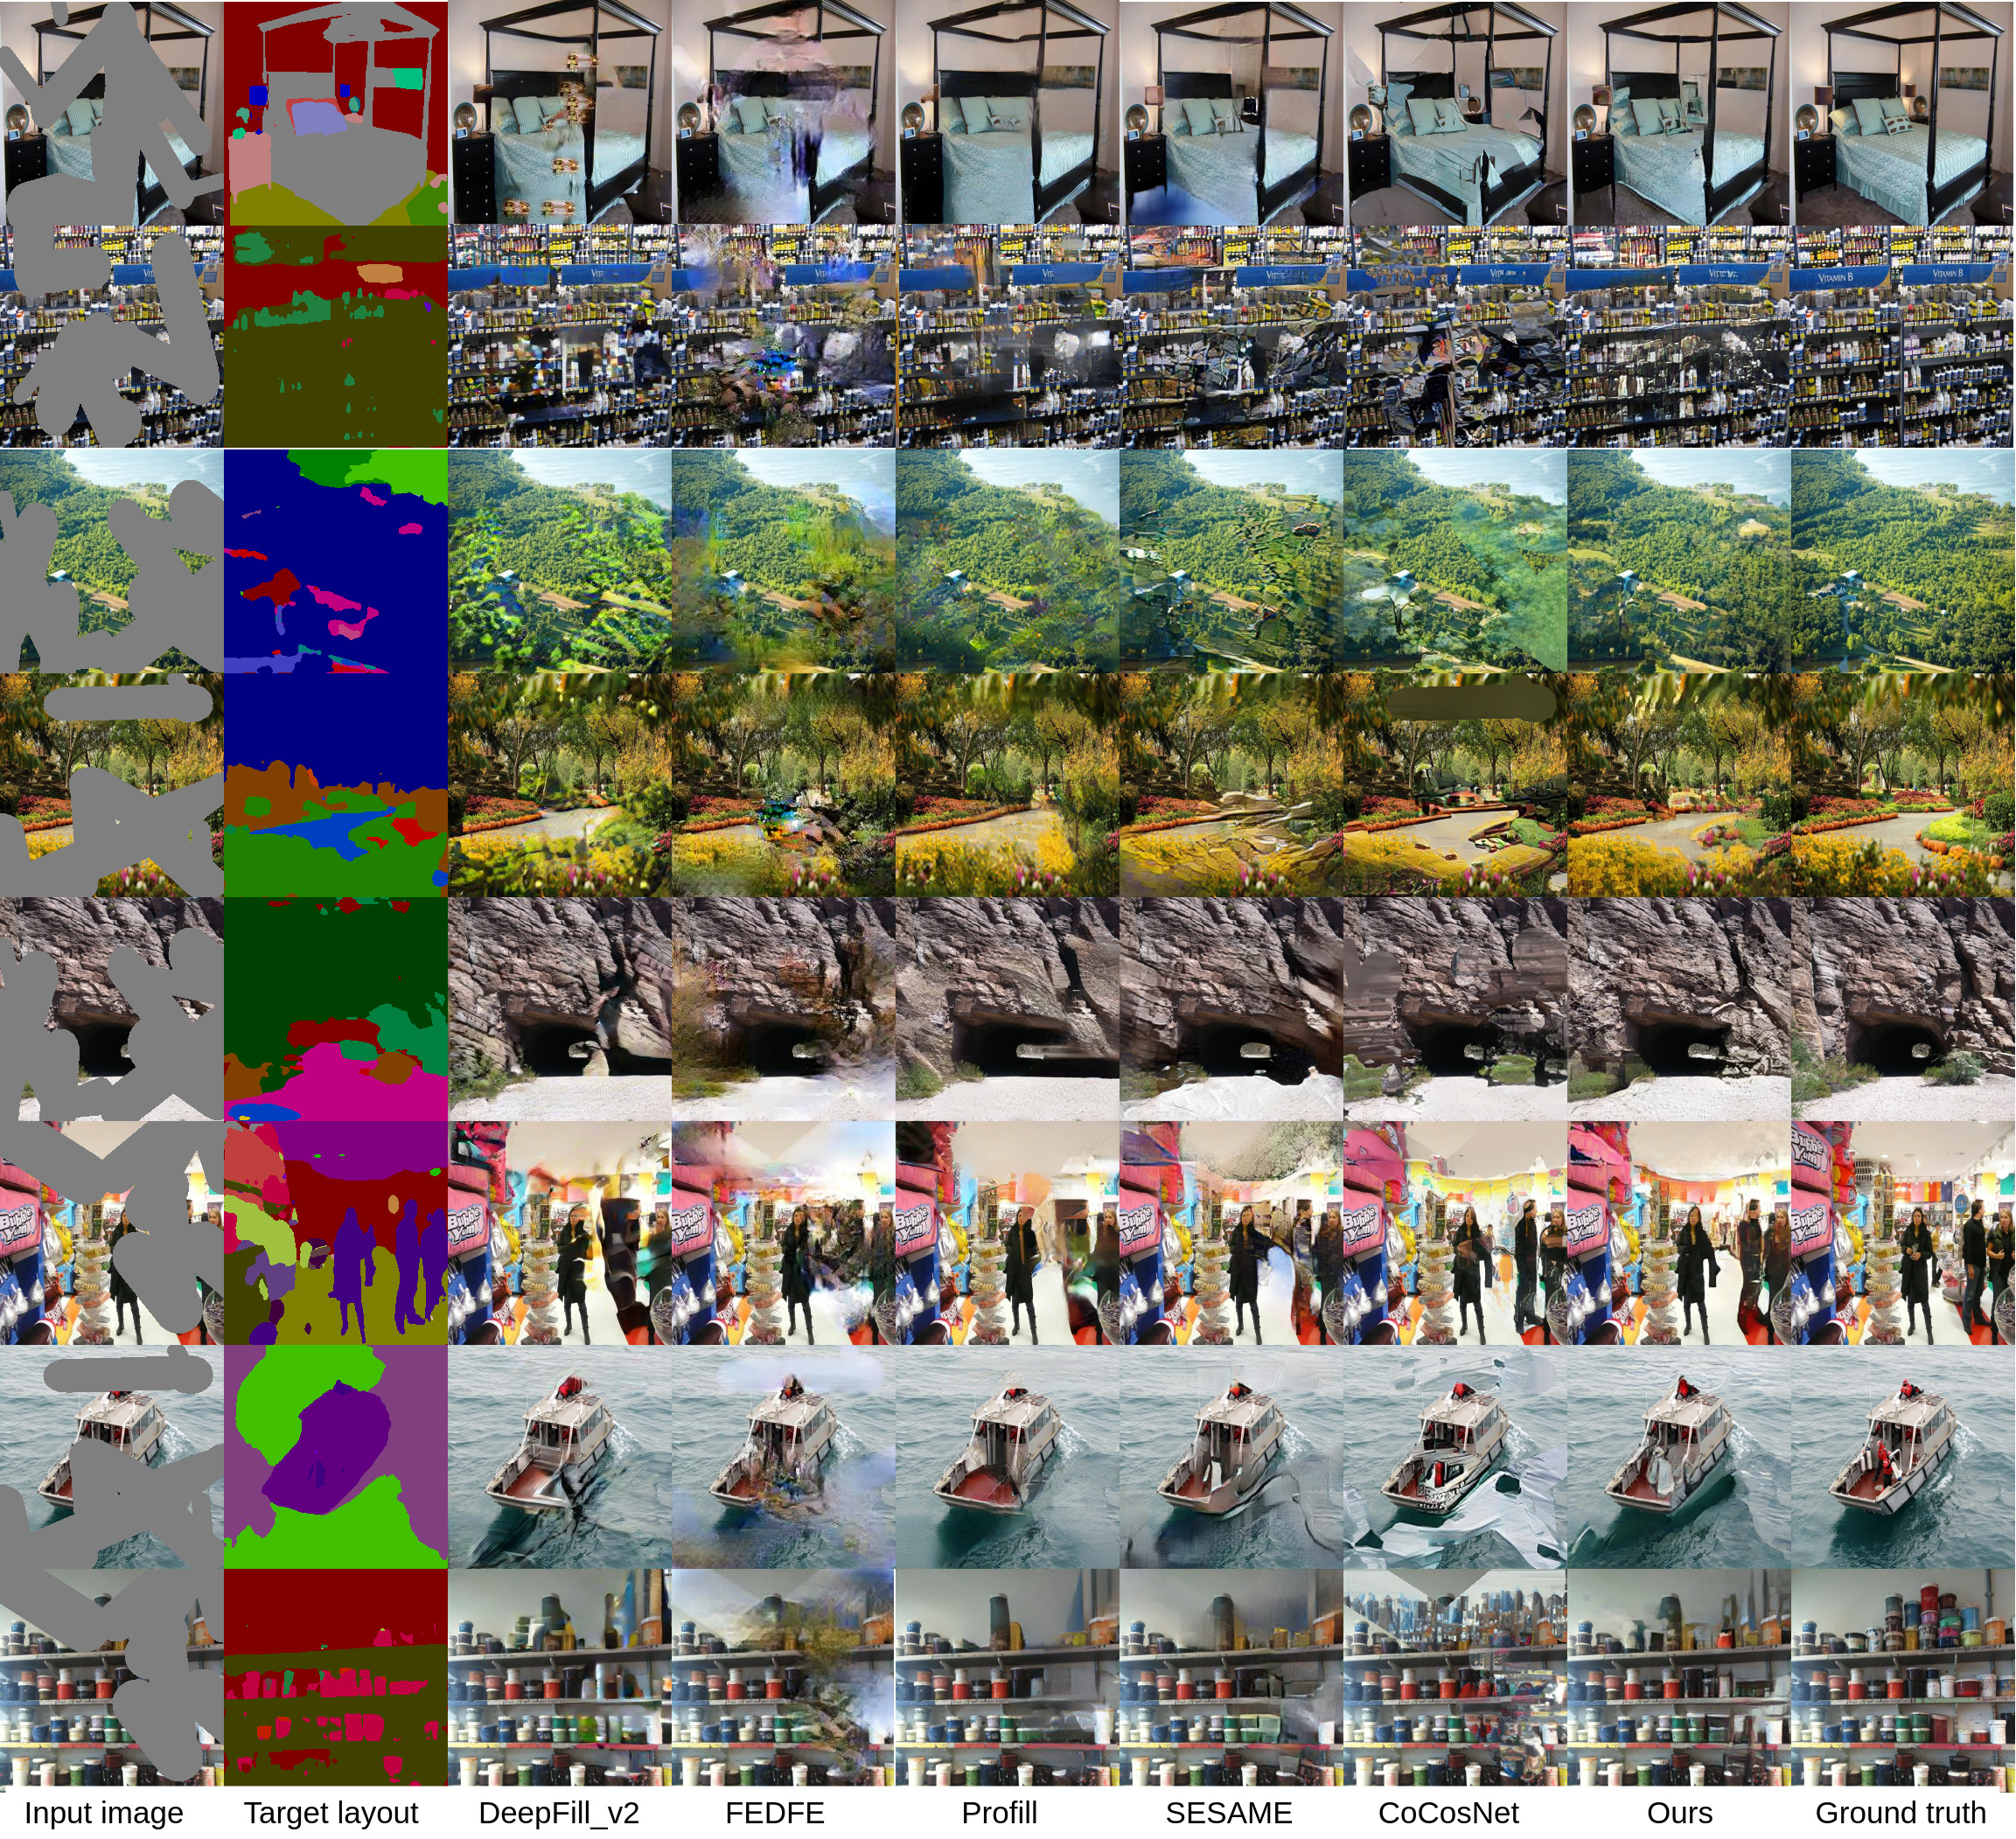}
	\caption{
	\textbf{Qualitative comparisons on the guided reconstruction task (Places365 dataset).} Best viewed (e.g. local textures) with zoom-in on screen.}
	\label{fig:compare_guided_inpainting}
\end{figure*}

\begin{figure*}[t]
	\centering
	\includegraphics[width=1.0\linewidth]{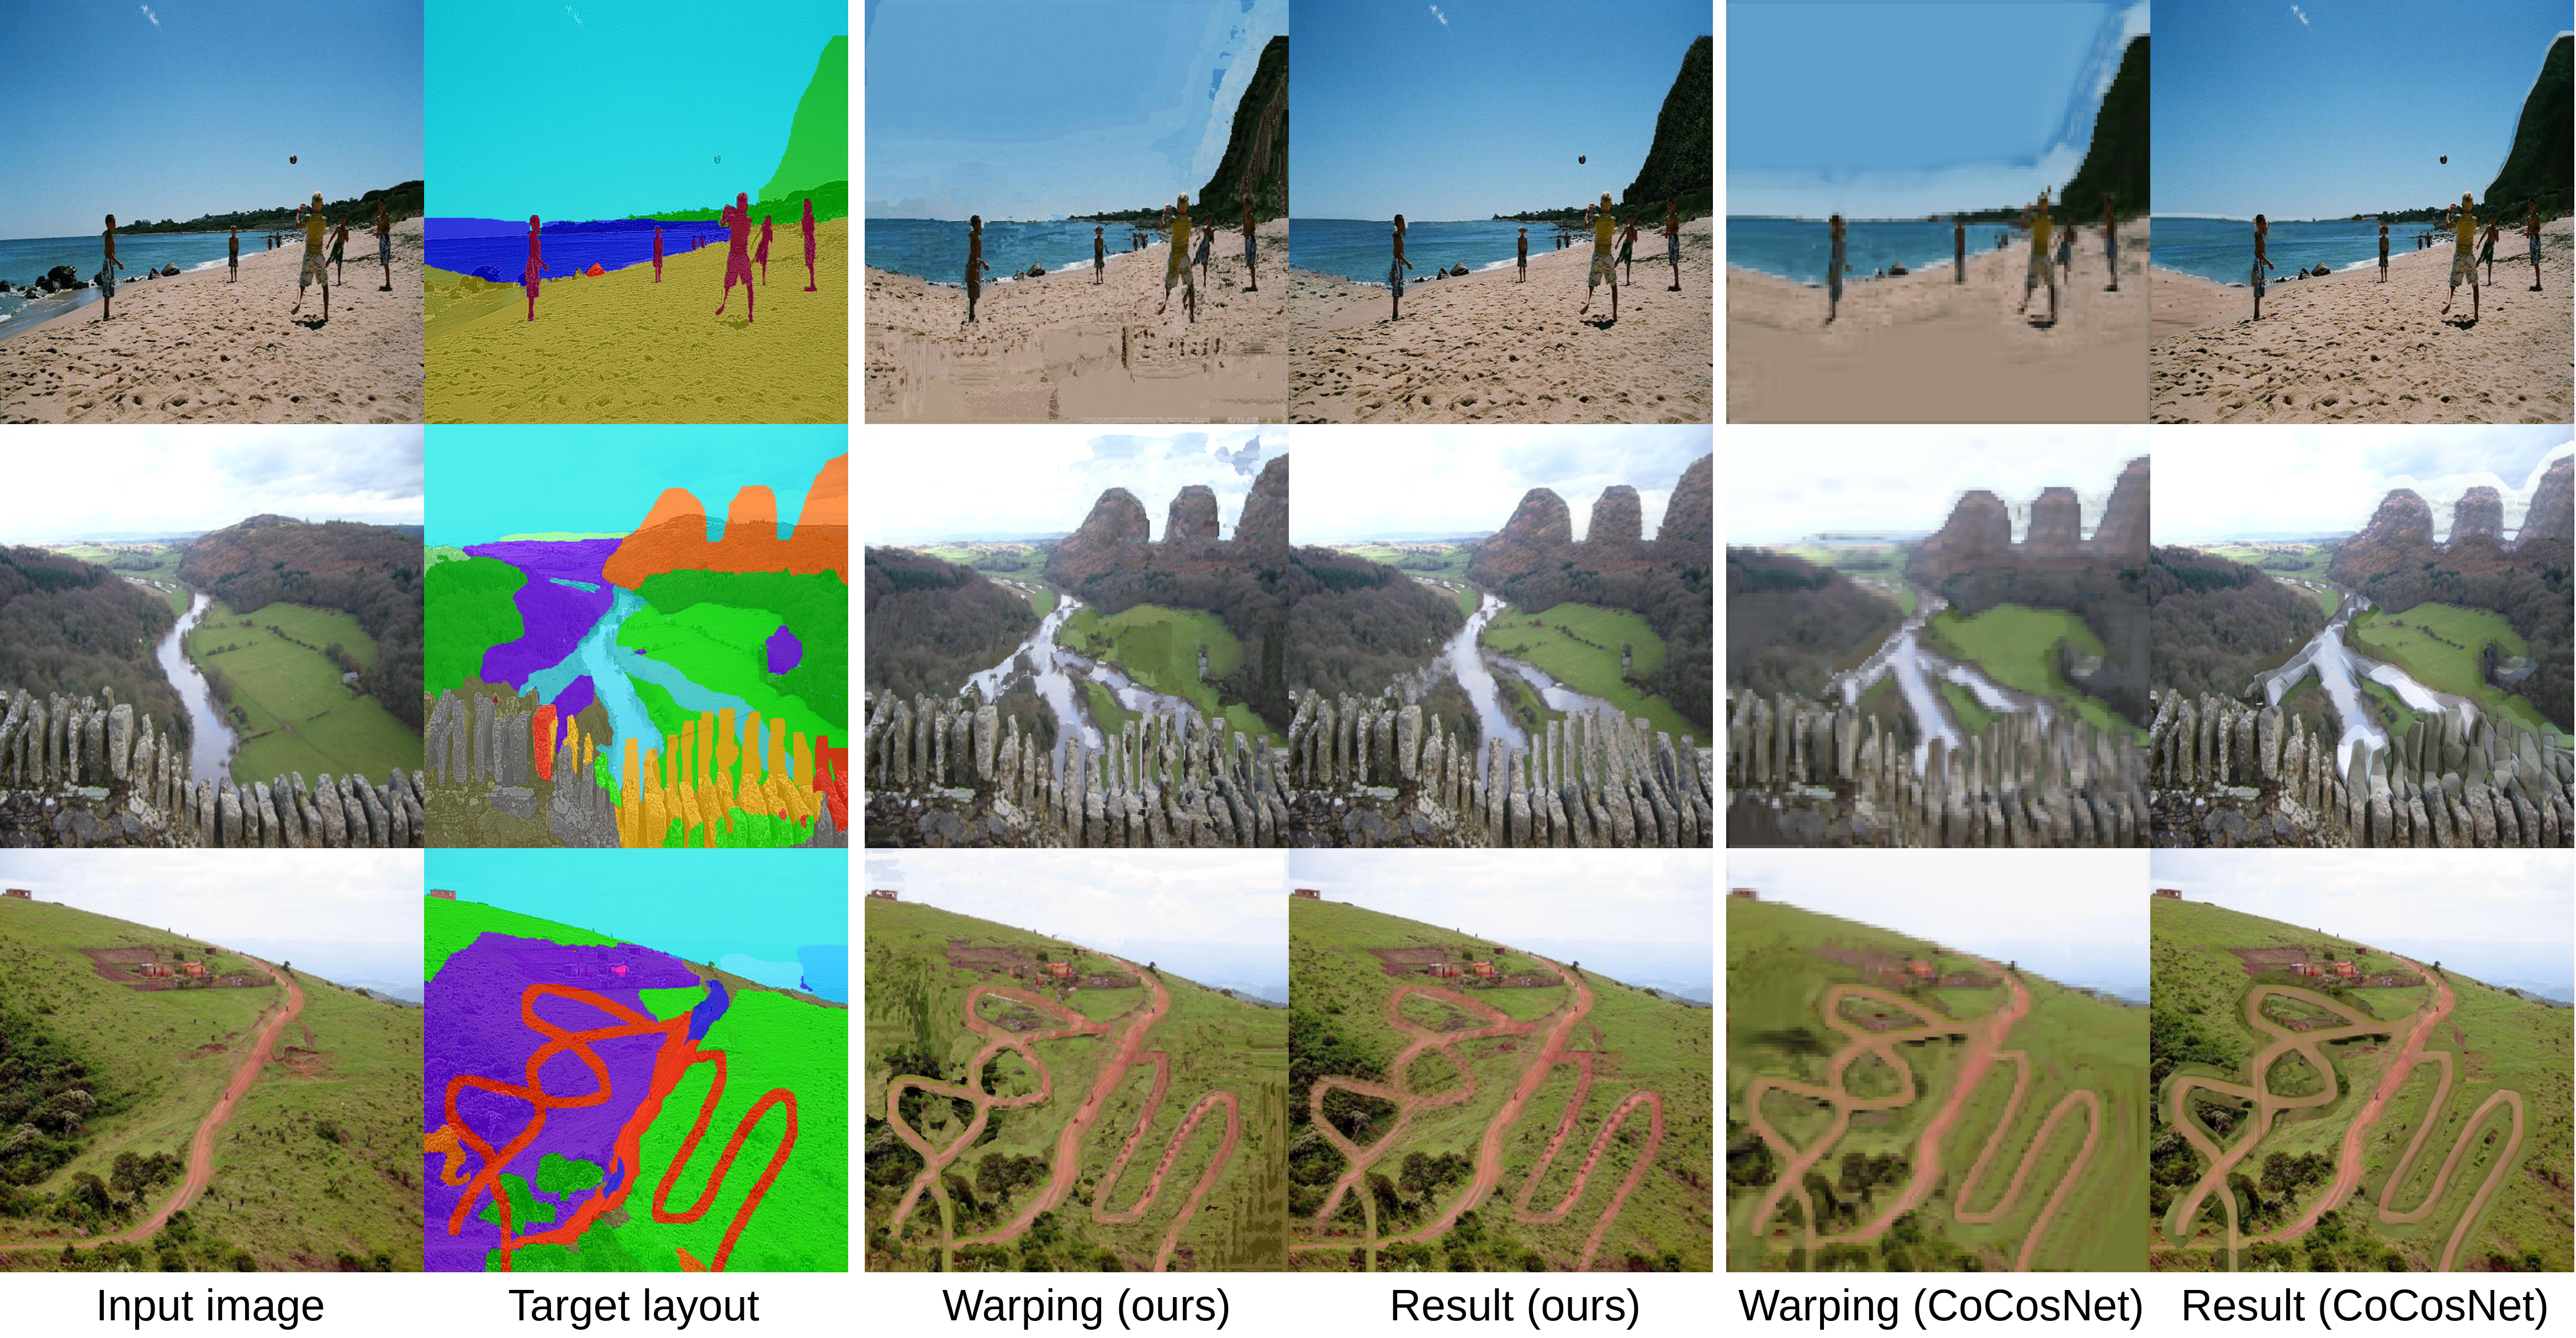}
	\caption{
	\textbf{Results on real manipulation data.} 
	Our model generate high-resolution warping results to facilitate detail-preserving manipulation.
	Best viewed (e.g. local textures) with zoom-in on screen.}
	\label{fig:compare_real_manipulation}
\end{figure*}

\section{More Results for Additional Reference-based Layout Manipulation Applications}

\label{sec:reference}
As shown in Fig.~\ref{fig:application} of the main paper, our method can also take additional reference images as input for semantic layout manipulation, multi-image warp compositing. In Fig.~\ref{fig:application1} to~\ref{fig:application5}, we show more results of our method for such applications including additional image editing use cases such as visual attribute editing, object insertion. Note that our method can re-synthesize and compose contents from multiple image sources to produce visually realistic generation consistent with the input layout.

\begin{figure*}[t]
	\centering
	\includegraphics[width=1.0\linewidth]{sections/figures/supp_application.png}
	\caption{
	\textbf{Object insertion via an additional reference image.}
	In addition to changing the layout of mountain (right),
	our method takes an additional reference image as input (left) to manipulate building and trees, and insert them into the new layout.}
	\label{fig:application1}
\end{figure*}

% \begin{figure*}[t]
% 	\centering
% 	\includegraphics[width=1.0\linewidth]{sections/figures/supp_application3.png}
% 	\caption{\textbf{Object insertion via an additional reference image.}
% 	In addition to editing the layout of mountain, 
% 	our method takes an additional reference image as input (left) to insert grass and trees.}
% 	\label{fig:application2}
% \end{figure*}

\begin{figure*}[t]
	\centering
	\includegraphics[width=1.0\linewidth]{sections/figures/supp_application2.png}
	\caption{
	\textbf{Attribute editing/transfer via an additional reference image.}
	Our method takes an additional reference image as input (left) to edit the texture and shape of the mountain (right).}
	\label{fig:application3}
\end{figure*}

\begin{figure*}[t]
	\centering
	\includegraphics[width=1.0\linewidth]{sections/figures/supp_application4.png}
	\caption{
	\textbf{Attribute editing/transfer via an additional reference image.}
	In addition to editing the layout of bush, 
	our method takes an additional reference image as input (left) to edit the texture and shape of the mountain (right).
	}
	\label{fig:application4}
\end{figure*}

\begin{figure*}[t]
	\centering
	\includegraphics[width=1.0\linewidth]{sections/figures/supp_application5.png}
	\caption{
	\textbf{Object shape manipulation and scene attribute editing via an additional reference image.}
	In addition to editing the shapes of objects including building and rock, 
	our method takes an additional reference image as input (left) to edit the textures of sky and trees in the background (right).
	}
	\label{fig:application5}
\end{figure*}

\section{Details of the Key Index Sampling Algorithm}
In this section, we elaborate the implementation details of the propagation and evaluation steps of the key index sampling algorithm.

\noindent \textbf{Propagation.} \quad The propagation step takes the particle coordinate map $\mathbf{t}$ as input and aims to propagated particles to $p$ from adjacent pixels of $p$. 
As described in~\cite{supp_duggal2019deeppruner}, such a propagation step essentially offsets the particle coordinates map to 4 directions, e.g. top, down, left and right by 1-pixel and can be efficiently implemented by  convolving the particle coordinates map with a predefined one-hot filter pattern. To propagate particles from 8-adjacent neighbors, we first apply propagation horizontally then apply propagation vertically.

\noindent \textbf{Evaluation.} \quad The function evaluation($\mathbf{t}, f_x^h, f_c^h,M$) aims to select the top $M$ matching particles from $\mathbf{t}(p)$ at location $p$ using the reference and content feature $f_x^h$ and $f_c^h$. To achieves this, we apply bilinear sampling~\cite{supp_stn} to warp the reference features $f_c^h$ to location defined by particle coordinate $\mathbf{t}$. Then we compute the matching score between the warped feature and the content features and select the top-$M$ particles accordingly.

\section{Optimization for Local Editing}
To achieve better local alignment for the semantic layout manipulation task, we optimize the key index sampling algorithm in several ways: 
\begin{enumerate}
    \item We modify the matching scores at each evaluation step such that matching for different semantic labels is penalized. To achieves this, we additionally warp the one-hot semantic label map and compute the $\ell_1$ distance between the warped label map and the content label map. Next, the negative distance is added to the feature matching score before the top-$M$ matching value selection.
    \item We perform particle sampling only in local windows around the position of the current particles where as the window size $w$ is also annealed in each iteration and decayed to zero. Specifically, $w=w_0 e^{-\lambda i} \mathbbm{1}(i<i_{t})$ where $w_0$ is the initial window size, $\lambda$ is the decay rate, $i$ is the iteration step and $i_{t}$ is a constant threshold term.
    \item We perform more propagation steps in each iteration of key index sampling to enforce spatial coherency.
\end{enumerate}

\section{Details of Sparse Attention Warping}
We take advantage of the modulated deformable convolution~\cite{supp_deformableConv} 
to implement the sparse attention warping. In particular, the modulated deformable convolution takes the following form:
\begin{align}
\label{eq:dcn}
\begin{aligned}
    y(p) = \sum_{k=1}^{K} w_k \cdot x(p+q_k+\Delta q_k) \cdot \Delta m_k,
\end{aligned}
\end{align}
where $q_k$ are offsets of the convolutional kernel, $\Delta q_k$ and $\Delta m_k$ are the offset and modulation factor for the k-th location. Since $p+q_k+\Delta q_k$ is fractional, ~\cite{supp_deformableConv} applies bilinear interpolation to compute $x(p+q_k+\Delta q_k)$.

To implement the sparse attention warping that weighted averages $x$ over all locations $S_k(\mathbb{C}_p)$ from the key index set $S(\mathbb{C}_p)$, we set $\Delta q_k=S_k(\mathbb{C}_p)-p-q_k$, $w_k$ to $1$ and $\Delta m_k$ to the computed softmax-normalized attentive weights.

\section{Details of the Guided Reconstruction Task}
The reconstruction task aims to reconstruct ground truth images from masked images using an semantic label map as guidance. 
As warping modules of our method and that of CoCosNet~\cite{supp_cocosnet} are designed to use pixels both inside and outside the mask, to make fair comparison with other inpainting methods, we modify our warping stage such that pixels inside the mask are explicitly ignored in the attention-based alignment stage. Specifically, we set large negative values to the correlation matrix of CoCosNet~\cite{supp_cocosnet} for the masked pixels to avoid warping pixels from inside the mask. Likewise, in the evaluation stage of our model, we set large negative values to the matching scores when matched pixels are from inside the mask.

\section{Other Experiments}
\subsection{User Study}
% \section{User Study}
To better evaluate visual quality of our method, we conduct a user study and show the result in Table~\ref{tab:ablation}.  Specifically, we randomly select 25 images from the Place365 validation set for manipulation and reconstruction, respectively. We show results of each image to 9 users and ask them to select the best results. Finally, we collect 225 votes from all users for each dataset. Results in the table show that our method receives the majority of the votes on both manipulation and reconstruction tasks.

\begin{table}[]
	\caption{User preference for the results of each method. 
	}
	\centering
% 	\resizebox{\columnwidth}{!}{
	\begin{tabular}{ |l|c|}
    %   \toprule
    %   \toprule
		\hline
		\hline
		Methods                             & Preference Votes\\
		\hline
		\multicolumn{2}{|l|}{\em Manipulation}\\
		\hline
		SESAME~\cite{supp_sesame}&  13\\
		CoCosNet~\cite{supp_cocosnet}&  14\\
		Ours&  198\\
		\hline
		\multicolumn{2}{|l|}{\em Reconstruction}\\
		\hline
		Deepfill\_v2~\cite{supp_deepfillv2}& 33 \\
		MEDFE~\cite{supp_liu2020rethinking}& 0\\
		Profill~\cite{supp_profill}& 23\\
		SESAME~\cite{supp_sesame}&  2\\
		CoCosNet~\cite{supp_cocosnet}&  3\\
		Ours&   164\\
		\hline
		\hline
	\end{tabular}
% 	}
	\label{tab:ablation}
\end{table}

\subsection{Comparisons Against Edge-connect~\cite{supp_edgeconnect} on the reconstruction task.}
We additionally show quantitative comparison against Edge-connect~\cite{supp_edgeconnect} on the reconstruction task in Table~\ref{tab:edge_connect}. The table shows that our method consistently outperforms Edge-connect by a large margin across all metrics.

\begin{table}[]
    \caption{Quantitative comparison against Edge-connect~\cite{supp_edgeconnect}. 
	}
	\centering
	\resizebox{\columnwidth}{!}{
	\begin{tabular}{ |l|c|c|c|c|c|c|}
    %   \toprule
    %   \toprule
		\hline
		\hline
		Methods                             &$\ell_1$ err. $\downarrow$ &	PSNR$\uparrow$ & SSIM$\uparrow$ &  LPIPS$\downarrow$	& FID$\downarrow$ & $\mathcal{L}_{style}$~\cite{supp_gatys2015neural}$\downarrow$\\
		\hline
		\multicolumn{7}{|l|}{\em ADE20k}\\
		\hline
		Edge-connect~\cite{supp_edgeconnect}&  0.04512&  20.179&  0.742 & 0.284& 80.96&6.061e-06\\
		Ours&  \best{0.02384}&  \best{23.048}&  \best{0.870} & \best{0.249}& \best{58.27}&\best{2.78e-06}\\
		\hline
		\multicolumn{7}{|l|}{\em Places365}\\
		\hline
		Edge-connect~\cite{supp_edgeconnect}&  0.05448&  19.158&  0.694 & 0.286& 97.21&6.517e-06\\
		Ours&   \best{0.05419}&  \best{19.177}&  \best{0.708} & \best{0.268}& \best{89.25} &\best{2.719e-06}\\
		\hline
		\hline
	\end{tabular}
	}
	\label{tab:edge_connect}
\end{table}

% {
% \small
% \bibliographystylesupp{ieee_fullname}
% \bibliographysupp{egbib2}
% }
